# Supplementary material for: Deep Learning Service for Efficient Data Distribution Aware Sorting
Source: arXiv:1907.08817 source file (2024-12-13)
Supplement: Supplementary file 1 [file appendix.tex]

 %!TEX root = paper.tex
%\newpage

%\twocolumn

%\renewcommand{\sstab}{\rule{0pt}{8pt}\\[-1.4ex]}
%\sloppy

%\def\baselinestretch{1.08}
%\addtolength{\parskip}{0.25cm}
\addtolength{\parskip}{0.18ex}

\newenvironment{ab}
  {\mathactivatecomma
   \mathcode`\,=\string"8000
   \ignorespaces}
  {\ignorespacesafterend}2

\newcommand{\mathactivatecomma}{%
  \begingroup\lccode`~=`\,
  \lowercase{\endgroup\edef~}{\mathchar\the\mathcode`\,\penalty0 }}

  \newcommand{\bab}{\begin{ab}}
  \newcommand{\eab}{\end{ab}\xspace}

\vspace{-1.7ex}
\section*{Appendix A: Proofs}
\vspace{-2ex}

\stitle{Proof of Corollary~\ref{thm-Church-Rosser}.}

\stitle{Proof of Theorem~\ref{thm-complexity}.} 
We prove that the 

\noindent
\etitle{Lower bound}. We next show that the problem is \NP-hard by reduction from the Boolean conjunctive query
 evaluation (BCQE) problem, which is known to be \NP-complete~\cite{CQ-Evaluation-NP}. The BCQE problem is to
  decide, given a conjunctive query $Q$ and a database $\D'$ of schema $\R'$, whether $Q(\D')$ is \true.

Given $Q$ and $\D'$, we construct a database schema $\R$, a database $\D$ of $\R$, a set $\Sigma$ of $\MRMLs$ 
over $\R$, a pair $(t_1.\id, t_2.\id)$ such that $Q(D')=\true$ if and only if $(t_1.\id, t_2.\id)$ is a match.
More specifically, (a)~ $\R$ consists of all relational schema in $\R'$ and an extra schema $S=(\id, A)$, 
(b)~$\D$ consists of all tuples of $\D'$ and two extra tuples $t$ and $t'$ of $S$ with $t.A=a$ and $t'.A=a'$ of $\R$, 
(c)~ $\Sigma$ consists of a single \MRML  $Q\wedge S(t)\wedge S(t')\rightarrow t.\id=t'.\id$, and (d)~$t$ and $t'$ are two tuples of $S$. 
One can readily verify that $Q(\D')$ is \true if and only if $(t.\id, t'.\id)$ is a match.
